# Supplementary material for: Deterministic and universal quantum squeezing gate in virtue of teleportation-like protocol
Source: arXiv:2202.07134 source file (2022-02-15)
Supplement: Supplementary file 1 [file Supporting_Information.pdf]

# Supporting Information for “Deterministic and universal quantum squeezing gate with a teleportation-like protocol”

Xiaocong Sun<sup>1</sup>, Yajun Wang<sup>1,2</sup>, Yuhang Tian<sup>1</sup>, Qingwei Wang<sup>1</sup>, Long Tian<sup>1,2</sup>, Yaohui Zheng<sup>1,2,\*</sup>, and Kunchi Peng<sup>1,2</sup>

<sup>1</sup>*State Key Laboratory of Quantum Optics Quantum Optics Devices, Institute of Opto-Electronics, Shanxi University, Taiyuan 030006, China*

<sup>2</sup>*Collaborative Innovation Center of Extreme Optics, Shanxi University, Taiyuan, 030006, China*

Additional information about “Deterministic and universal quantum squeezing gate with a teleportation-like protocol” is as follows: Sec. I, Selection of the scaling factors. Sec. II, Theoretical model of the quantum squeezing gate. Sec. III, Generation of entangled Einstein-Podolsky-Rosen (EPR) beam. Sec. IV, Analysis of complex quantum operation. Sec. V, Scheme of a heralded quantum squeezing gate.

## I. Selection of the scaling factors

The scaling factors are the suitably normalized gains for the amplitude  $\hat{X}$  and phase  $\hat{P}$  quadratures, through which the measured classical information from homodyne detections (HOMs) are sent to the displaced field. In terms of the model given in Sec. II, the gains  $g_x$  and  $g_y$  are given explicitly by

$$g_x = \frac{1}{\sqrt{(1-R_D)(1-R)}} \quad (1.1)$$

$$g_y = \frac{1}{\sqrt{(1-R_D)R}} \quad (1.2)$$

Here  $R$  is reflectivity of variable beam splitter (VBS),  $R_D$  is reflectivity of 99/1 BS ( $R_D=0.99$ ). The convention for optimizing proper gain is adopt with following condition

$$\langle \hat{X}_{out} \rangle = \sqrt{\frac{R}{1-R}} \langle \hat{X}_{in} \rangle \quad (1.3)$$

$$\langle \hat{P}_{out} \rangle = \sqrt{\frac{1-R}{R}} \langle \hat{P}_{in} \rangle \quad (1.4)$$

Where  $\langle \hat{X} \rangle$  and  $\langle \hat{P} \rangle$  denote the expectation values of amplitude and phase

quadratures. The input-output relations in Eq. (1.3) and (1.4) are the unity-gain condition, which confirm that the transformation process is a unity operation. Then the optimal reconstruction of input state with arbitrary ancillary EPR entanglement can be achieved under this condition. The quantum squeezing gate is under unit-gain condition to justify its universality.

## II. Theoretical model of the quantum squeezing gate

Quantum states of light can be described by the electromagnetic field annihilation operator  $\hat{a} = (\hat{X} + i\hat{P})/\sqrt{2}$  with the canonical commutator  $[\hat{X}, \hat{P}] = i(\hbar = 1)$ .  $\hat{X}$  and  $\hat{P}$  are the associated amplitude and phase quadratures.

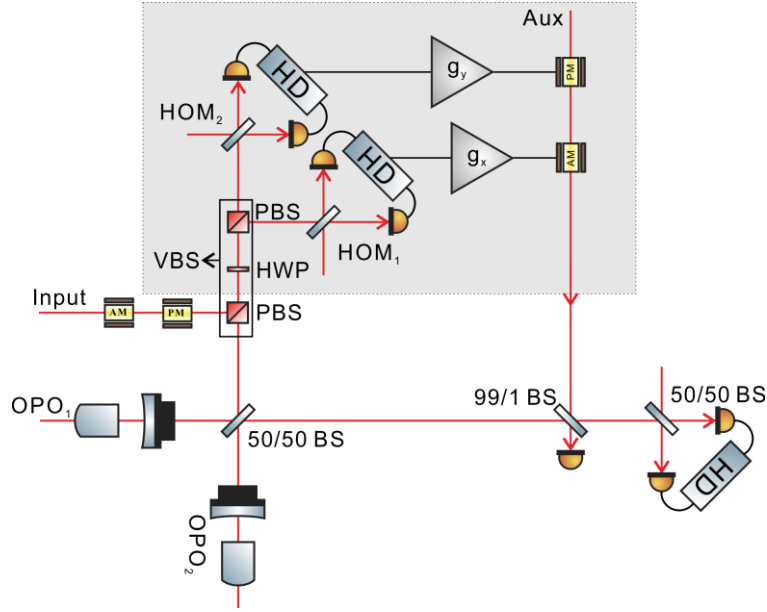

Fig. 1. Experimental setup of one-mode off-line scheme with an entangled state. OPO: optical parametric oscillator; BS: beam splitter; HWP: half wave plate; PBS: polarization beam splitter; VBS: variable beam splitter; HR: high reflectivity mirror; AM: amplitude modulator; PM: phase modulator; HOM: homodyne detection; Aux: auxiliary beam.

The scheme of one-mode off-line scheme with an EPR entangled state is illustrated in Fig. 1. The input state is combined with one half of EPR beam with the relative phase of 0 at a variable beam splitter (VBS), which is realized by a half-wave plate and two polarization beam splitters, the two outcomes in the Heisenberg picture can be derived as

$$\hat{a}_r = \sqrt{R}\hat{a}_{in} + \sqrt{1-R}\hat{a}_{EPR1} \quad (2.1)$$

$$\hat{a}_t = \sqrt{1-R}\hat{a}_{in} - \sqrt{R}\hat{a}_{EPR1} \quad (2.2)$$

Where  $R$  is the reflectivity of VBS.  $\hat{a}_r$  and  $\hat{a}_t$  represent the reflected and transmitted

field, respectively.  $\hat{a}_{in}$  is the input state.  $\hat{a}_{EPR1}$  is half of the EPR entangled state. The amplitude and phase quadrature noises are measured by two homodyne detections (HOMs), and the measured angles are 0 and  $\pi/2$ , respectively. The measured quadratures can be expressed as:

$$\hat{X}_m = \sqrt{R}\hat{X}_{in} + \sqrt{1-R}\hat{X}_{EPR1} \quad (2.3)$$

$$\hat{P}_m = \sqrt{1-R}\hat{P}_{in} - \sqrt{R}\hat{P}_{EPR1} \quad (2.4)$$

Where  $\hat{X}$  and  $\hat{P}$  are amplitude and phase quadrature operators.

The measurement outcomes are rescaled by gain factors denoted by  $g_x$  (for amplitude quadrature) and  $g_y$  (for phase quadrature), and then used to displace the system by an auxiliary beam (Aux). The displaced field combined with the other half of the EPR entanglement  $\hat{a}_{EPR2}$  at 99/1 BS ( $R_D=0.99$ ) is transmitted to the output

station, where the relative phase is 0. Considering gain factors  $g_x = \frac{1}{\sqrt{(1-R_D)(1-R)}}$

and  $g_y = \frac{1}{\sqrt{(1-R_D)R}}$ , we can arrive at the following input-output relation:

$$\begin{pmatrix} \hat{X}_{out} \\ \hat{P}_{out} \end{pmatrix} = \begin{pmatrix} \sqrt{\frac{R}{1-R}} & 0 \\ 0 & \sqrt{\frac{1-R}{R}} \end{pmatrix} \begin{pmatrix} \hat{X}_{in} \\ \hat{P}_{in} \end{pmatrix} + \begin{pmatrix} \hat{X}_{EPR1} + \hat{X}_{EPR2} \\ -\hat{P}_{EPR1} + \hat{P}_{EPR2} \end{pmatrix} \quad (2.5)$$

Where  $\hat{X}_{EPR1} + \hat{X}_{EPR2}$  and  $-\hat{P}_{EPR1} + \hat{P}_{EPR2}$  are the excess noise from amplitude and phase quadratures of the EPR entangled state, respectively, which result from the imperfect resource of entanglement state.

The single-mode amplitude or phase squeezing gate is implemented with

$\sqrt{\frac{R}{1-R}} = e^{-r_t}$  and  $e^{r_t}$ , where  $r_t$  is the squeezing parameter of target squeezing. We can

find that the output state is an amplitude squeezing gate with  $R < 1/2$  or a phase squeezing gate with  $R > 1/2$ , then the noise variances of output state can be expressed to be

$$V(\hat{X}_{out}) = \frac{R}{1-R} V(\hat{X}_{in}) + \delta^2(\hat{X}_{EPR1} + \hat{X}_{EPR2}) \quad (2.6)$$

$$V(\hat{P}_{out}) = \frac{1-R}{R} V(\hat{P}_{in}) + \delta^2 (-\hat{P}_{EPR1} + \hat{P}_{EPR2}) \quad (2.7)$$

The noise variances depend on correlated characteristic of the EPR beams. For an ideal EPR state,  $\hat{X}_{EPR1} + \hat{X}_{EPR2} = -\hat{P}_{EPR1} + \hat{P}_{EPR2} = 0$ , the transformation corresponds to an ideal quantum squeezing gate, which can be expressed as follows

$$V_{ideal}(\hat{X}_{out}) = \frac{R}{1-R} V(\hat{X}_{in}) \quad (2.8)$$

$$V_{ideal}(\hat{P}_{out}) = \frac{1-R}{R} V(\hat{P}_{in}) \quad (2.9)$$

For an input coherence state, the fidelity can be expressed by

$$F = \frac{2}{\sqrt{(V_{ideal}(\hat{X}_{out}) + V(\hat{X}_{out}))(V_{ideal}(\hat{P}_{out}) + V(\hat{P}_{out}))}} \\ = \frac{1}{\sqrt{(\frac{R}{1-R} + e^{-2r})(\frac{1-R}{R} + e^{-2r})}} \quad (2.10)$$

Where the subscripts “*ideal*” and “*out*” denote the ideal squeezing and the experimental output, respectively.  $V$  represents the variances of that.  $e^{-2r}$  denotes correlated characteristic of EPR beam with the squeezing parameter  $r$ . The unit fidelity can be achieved at arbitrary target squeezing for ideal EPR state with  $r \rightarrow \infty$ . The ideal EPR state does not exist really since it requires infinite energy.

### III. Generation of entangled Einstein-Podolsky-Rosen (EPR)

beam

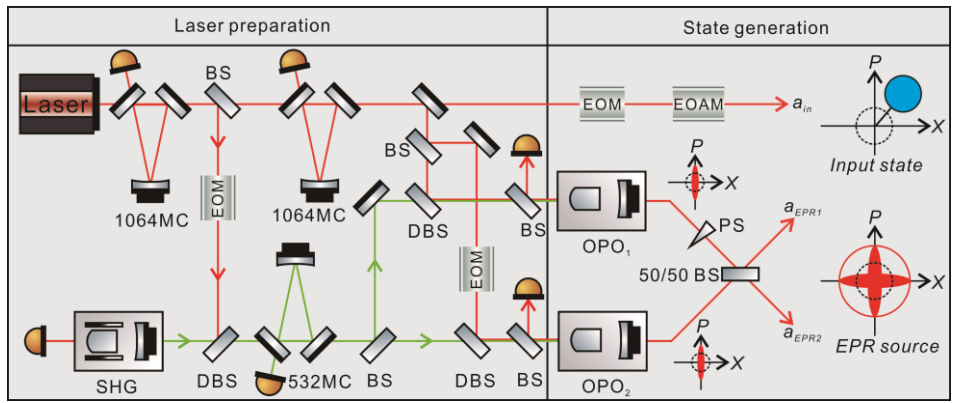

Fig. 2. Schematic of the entangled EPR beam generation. MC, mode cleaner; BS, beam splitter; DBS, dichroic beam splitter; EOM, electro-optical modulator; EOAM, electro-optical amplitude modulator; SHG, second harmonic generation; OPO, optical parametric oscillator; PS, phase shifter.

Schematic for the generation of the entangled EPR beams is illustrated in Fig. 2. In

the preparation stage, we need to generate the input state and the auxiliary EPR entanglement state. The laser is a home-made single-frequency laser at 1064 nm. Three mode cleaners (MC) are used to improve the properties of the laser beams, including the intensity noise and spatial distribution. The MCs ensure the quadrature noises of the fundamental and pump beams meet the shot noise limit (SNL) above 2 MHz at all power levels. The input coherent states are created by impinging 3MHz sidebands on a laser beam with an electro-optical phase and an electro-optical amplitude modulators. The residual power of the laser is divided into two parts. The most power is used for the second harmonic generation (SHG) to provide the pump field at 532 nm for our optical parameter oscillator (OPOs), and the other part is for seed beams. Generation of the entangled EPR beams consists of two OPOs with type-I phase-matching nonlinear crystal. The two OPOs are semi-monolithic single-resonant standing wave cavities, consisting of a piezo-actuated concave mirror and a periodically poled KTiOPO<sub>4</sub> (PPKTP) crystal with a dimension of 1mm×2mm×10mm. One end face of the crystal with a radius of curvature of 12 mm is coated as high reflectivity for the fundamental field and high transmission for the pump field, thus serving as a cavity end mirror. The plane front face is coated as antireflectivity for both wavelengths. An air gap of 27 mm length is realized between the plane face and the coupling mirror. The concave mirror with a radius of curvature of 30 mm has a transmissivity of 12% for 1064 nm and HR for 532 nm, which serves as the output coupler. The OPO cavity is locked on resonance with the fundamental beam (1,064 nm) by means of the Pound–Drever–Hall technique, with a 56.4 MHz (OPO1) and 34.8 MHz (OPO2) phase modulation on the seeds [1]. The relative phase between the seed and pump beam is carefully controlled to  $\pi$  for the requirement of parametric de-amplification, i.e., amplitude squeezed state. Detailed information for the generation of the squeezed states had been illustrated in Ref. [2, 3, 4]. Compared with the level of squeezing in Ref. [5, 6], 13.8 dB squeezed vacuum states below the shot noise limit (SNL) was directly measured in our scheme [3]. After the production of the two single mode states, they are directed toward a balanced beam splitter to produce the EPR entangled beams with a relative phase of  $\pi/2$ .

Here, we suppose that there are two single mode squeezed states with the same squeezing factors  $r$ , which can be expressed as

$$S_1 = \hat{a}_1 \cosh r - \hat{a}_1^\dagger \sinh r \quad (3.1)$$

$$S_2 = \hat{a}_2 \cosh r - \hat{a}_2^\dagger \sinh r \quad (3.2)$$

Where  $\hat{a}_1$  and  $\hat{a}_2$  are the annihilation operators of the two squeezed states. The two squeezed states are coupled on a 50/50 beam splitter with the relative phase of  $\pi/2$ . The output beams are entangled, which can be expressed as

$$E_1 = \frac{\sqrt{2}}{2}(S_1 + iS_2) = \frac{\sqrt{2}}{2}(\hat{a}_1 \cosh r - \hat{a}_1^\dagger \sinh r + i\hat{a}_2 \cosh r - i\hat{a}_2^\dagger \sinh r) \quad (3.3)$$

$$E_2 = \frac{\sqrt{2}}{2}(S_1 - iS_2) = \frac{\sqrt{2}}{2}(\hat{a}_1 \cosh r - \hat{a}_1^\dagger \sinh r - i\hat{a}_2 \cosh r + i\hat{a}_2^\dagger \sinh r) \quad (3.4)$$

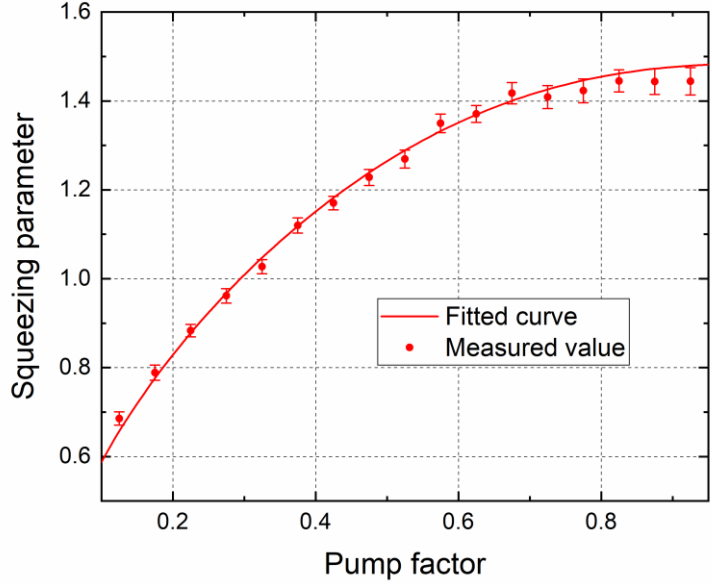

Fig. 3. Dependence of the squeezing parameter on the pump factor (ratio of the pump power to the threshold power). The separated dot is the measured result in the experiment, the solid line is the fitted curve.

The squeezing parameter  $r$  is measured under different OPO pump factors (ratio of the pump power to the threshold power), which is shown in Fig. 3. The threshold power of the OPO1 is about 163 mW and 193 mW that of OPO2. The dependence of the squeezing parameter  $r$  on the pump factor is no obvious difference between the two OPOs. Ideally, the squeezing factor of the generated entanglement state has the same value as the originally squeezed states, which reaches the maximum value at the threshold power of 80%. Here, in order to reduce the influence of anti-correlation noise on the fidelity, both of the two OPOs operate at the threshold power of 65%, where 12 dB-entangled EPR beams are experimentally produced by taking into account the additional propagation loss.

#### IV. Analysis of complex quantum operation

The input state is combined with half of the EPR entanglement at a VBS with a relative phase of  $\pi/2$ , consisting of a half-wave plate and two polarization beam splitters, the two outcomes in the Heisenberg picture can be derived

$$\hat{a}_r = \sqrt{R}\hat{a}_{in} + e^{i\theta_0}\sqrt{1-R}\hat{a}_{EPR1} \quad (4.1)$$

$$\hat{a}_t = \sqrt{1-R}\hat{a}_{in} - e^{i\theta_0}\sqrt{R}\hat{a}_{EPR1} \quad (4.2)$$

Where  $R$  is the reflectivity of the VBS,  $\theta_0 = \frac{\pi}{2}$  is the relative phase between the input state and  $\hat{a}_{EPR1}$ . The quadratures in Eq. (4.1) and (4.2) can be also expressed as:

$$\hat{X}_{m1} = \sqrt{R}\hat{X}_{in} - \sqrt{1-R}\hat{P}_{EPR1} \quad (4.3)$$

$$\hat{P}_{m1} = \sqrt{R}\hat{P}_{in} + \sqrt{1-R}\hat{X}_{EPR1} \quad (4.4)$$

$$\hat{X}_{m2} = \sqrt{1-R}\hat{X}_{in} + \sqrt{R}\hat{P}_{EPR1} \quad (4.5)$$

$$\hat{P}_{m2} = \sqrt{1-R}\hat{P}_{in} - \sqrt{R}\hat{X}_{EPR1} \quad (4.6)$$

Where  $\hat{X}_{m1}$  and  $\hat{P}_{m1}$  represent the amplitude and phase quadratures of the reflected field, and  $\hat{X}_{m2}$  and  $\hat{P}_{m2}$  represent amplitude and phase quadratures of the transmitted field.

The amplitude and phase quadrature noises are measured by the two homodyne detections HOM<sub>1</sub> and HOM<sub>2</sub>. The measured angles are  $\theta_1$  and  $\theta_2$ , respectively. The measured outcomes can be expressed as:

$$\hat{X}_m = \hat{X}_{m1} \cos \theta_1 + \hat{P}_{m1} \sin \theta_1 \quad (4.7)$$

$$\hat{P}_m = \hat{X}_{m2} \cos \theta_2 + \hat{P}_{m2} \sin \theta_2 \quad (4.8)$$

#### A. Fourier operation

Considering  $\theta_1 = \pi/2$ ,  $\theta_2 = \pi$ , then the input-output relation can be expressed by

$$\begin{pmatrix} \hat{X}_{out} \\ \hat{P}_{out} \end{pmatrix} = \begin{pmatrix} 0 & \sqrt{\frac{R}{1-R}} \\ -\sqrt{\frac{1-R}{R}} & 0 \end{pmatrix} \begin{pmatrix} \hat{X}_{in} \\ \hat{P}_{in} \end{pmatrix} + \begin{pmatrix} \hat{X}_{EPR1} + \hat{X}_{EPR2} \\ -\hat{P}_{EPR1} + \hat{P}_{EPR2} \end{pmatrix} \quad (4.9)$$

Where  $R$  is the reflectivity of VBS. The gain factors are chosen to be

$g_x = \frac{1}{\sqrt{(1-R_d)(1-R)}}$  and  $g_y = \frac{1}{\sqrt{(1-R_d)R}}$ , respectively. The transformation matrix

$\begin{pmatrix} 0 & 1 \\ -1 & 0 \end{pmatrix}$  corresponds to a fully Fourier operation with  $R=1/2$ . In addition, the results

show that a complex amplitude squeezing and Fourier operation is implemented simultaneously with  $R < 1/2$ , or a complex phase squeezing and Fourier gate with  $R > 1/2$ . It means our device can easily realize the complex quantum logical operation and used for universal single-mode quantum computation.

## B. Rotation operation

Considering  $\theta_1 = -\theta_2 = \theta$ , then the input-output relation can be expressed by

$$\begin{pmatrix} \hat{X}_{out} \\ \hat{P}_{out} \end{pmatrix} = \begin{pmatrix} (g_{X1}\sqrt{R} + g_{Y1}\sqrt{1-R})\cos\theta & (g_{X1}\sqrt{R} - g_{Y1}\sqrt{1-R})\sin\theta \\ (g_{X2}\sqrt{R} + g_{Y2}\sqrt{1-R})\cos\theta & (g_{X2}\sqrt{R} - g_{Y2}\sqrt{1-R})\sin\theta \end{pmatrix} \begin{pmatrix} \hat{X}_{in} \\ \hat{P}_{in} \end{pmatrix} \\ + \begin{pmatrix} (g_{X1}\sqrt{1-R} + g_{Y1}\sqrt{R})\sin\theta \hat{X}_{EPR1} + \hat{X}_{EPR2} + (g_{Y1}\sqrt{R} - g_{X1}\sqrt{1-R})\cos\theta \hat{P}_{EPR1} \\ (-g_{X2}\sqrt{1-R} + g_{Y2}\sqrt{R})\cos\theta \hat{P}_{EPR1} + \hat{P}_{EPR2} + (g_{X2}\sqrt{1-R} + g_{Y2}\sqrt{R})\sin\theta \hat{X}_{EPR1} \end{pmatrix} \quad (4.10)$$

For a complex rotation and quantum squeezing gate, the output state is

$$\begin{pmatrix} \hat{X}_{out} \\ \hat{P}_{out} \end{pmatrix} = \frac{1}{2} \begin{pmatrix} (\sqrt{\frac{R}{1-R}} + \sqrt{\frac{1-R}{R}})\cot\theta & (\sqrt{\frac{R}{1-R}} - \sqrt{\frac{1-R}{R}}) \\ (\sqrt{\frac{R}{1-R}} - \sqrt{\frac{1-R}{R}}) & (\sqrt{\frac{R}{1-R}} + \sqrt{\frac{1-R}{R}})\tan\theta \end{pmatrix} \begin{pmatrix} \hat{X}_{in} \\ \hat{P}_{in} \end{pmatrix} + \begin{pmatrix} \hat{X}_{EPR1} + \hat{X}_{EPR2} \\ -\hat{P}_{EPR1} + \hat{P}_{EPR2} \end{pmatrix} \quad (4.11)$$

Where  $g_{X1} = \frac{1}{2\sqrt{1-R}\sin\theta}$ ,  $g_{Y1} = \frac{1}{2\sqrt{R}\sin\theta}$ ,  $g_{X2} = \frac{1}{2\sqrt{1-R}\cos\theta}$ ,  $g_{Y2} = \frac{-1}{2\sqrt{R}\cos\theta}$ .

Clearly, from Eq. (4.11), the complex squeezing and Fourier operations at different target squeezing can be experimental performed with the measured quadrature angles of the HOMs varied. The fidelity of the complex operation is limited by ancilla EPR entanglement. Furthermore, the level of target squeezing can be tuned by varying the reflectivity  $R$ , and rotation operation in phase space is achieved by changing the measured quadrature angles of HOMs, and it is much easier to be implemented with the two freedom variables compared with the conventional schemes [7, 8].

## V. Scheme of a heralded quantum squeezing gate

### A. Scheme of a heralded quantum squeezing gate based on ancillary EPR entanglement.

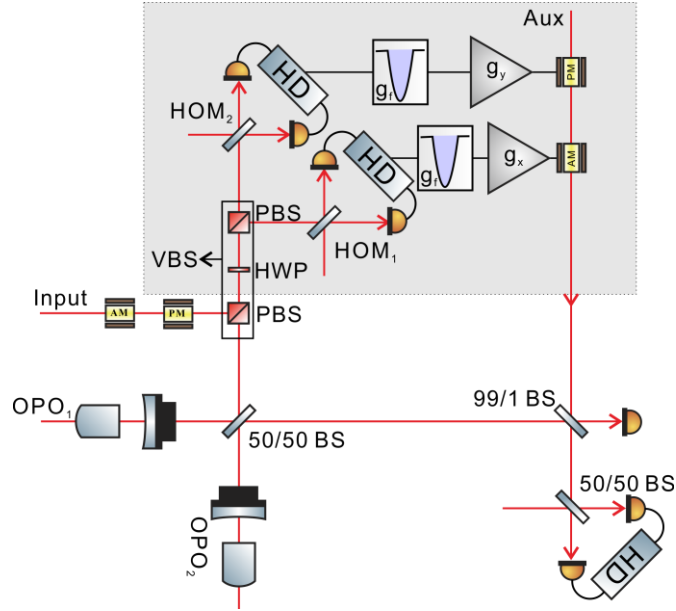

Fig. 4. Scheme for a heralded quantum squeezing gate with ancillary EPR entanglement.

Fig. 4 shows a scheme for heralded quantum squeezing gate based on entanglement. An input state is coupled with half of a bipartite EPR entanglement  $\hat{a}_{EPR1}$  at a VBS, that is

$$\hat{a}_r = \sqrt{R}\hat{a}_{in} + \sqrt{1-R}\hat{a}_{EPR1} \quad (5.1)$$

$$\hat{a}_t = \sqrt{1-R}\hat{a}_{in} - \sqrt{R}\hat{a}_{EPR1} \quad (5.2)$$

Then the reflected and transmitted parts are measured by the two HOMs

$$\hat{X}_m = \sqrt{R}\hat{X}_{in} + \sqrt{1-R}\hat{X}_{EPR1} \quad (5.3)$$

$$\hat{P}_m = \sqrt{1-R}\hat{P}_{in} - \sqrt{R}\hat{P}_{EPR1} \quad (5.4)$$

We can express the other half of the bipartite entanglement  $\hat{a}_{EPR2}$  as a function of the measured quadrature  $(\hat{X}_m, \hat{P}_m)$  via

$$\hat{X}_{EPR2} = c\hat{X}_m + x + \hat{X}_n \quad (5.5)$$

$$\hat{P}_{EPR2} = d\hat{P}_m + y + \hat{P}_n \quad (5.6)$$

Where

$$c = \frac{\sqrt{1-R} * V(\hat{X}_{EPR1}, \hat{X}_{EPR2})}{V(\hat{X}_m)} \quad (5.7)$$

$$x = -c \langle \hat{X}_m \rangle \quad (5.8)$$

$$\langle \hat{X}_m \rangle = \sqrt{R} \hat{X}_{in} \quad (5.9)$$

$$V(\hat{X}_n) = V(\hat{X}_{EPR2}) - c^2 * V(\hat{X}_m) \quad (5.10)$$

$$V(\hat{X}_m) = R + (1 - R) * V(\hat{X}_{EPR1}) \quad (5.11)$$

$$d = \frac{\sqrt{R} * V(\hat{P}_{EPR1}, \hat{P}_{EPR2})}{V(\hat{P}_m)} \quad (5.12)$$

$$y = -d \langle \hat{P}_m \rangle \quad (5.13)$$

$$\langle \hat{P}_m \rangle = \sqrt{1 - R} y_{in} \quad (5.14)$$

$$V(\hat{P}_n) = V(\hat{P}_{EPR2}) - d^2 * V(\hat{P}_m) \quad (5.15)$$

$$V(\hat{P}_m) = 1 - R + R * V(\hat{P}_{EPR1}) \quad (5.16)$$

After that, we implement the noiseless linear amplifier (NLA) operation on the measured outcomes of  $\hat{X}_m$  and  $\hat{P}_m$ . Then we transform  $\hat{X}_m$  into  $\hat{X}_m^{NLA}$  and  $\hat{P}_m$  into  $\hat{P}_m^{NLA}$ :  $\langle \hat{X}_m^{NLA} \rangle = g_f * \langle \hat{X}_m \rangle$ ,  $\hat{X}_m^{NLA} = g_f * \hat{X}_m$ ,  $\langle \hat{P}_m^{NLA} \rangle = g_f * \langle \hat{P}_m \rangle$ ,  $\hat{P}_m^{NLA} = g_f * \hat{P}_m$ .

Finally, the rescaled signal is feedback into the amplitude modulator and phase modulator to displacement field, and the final outputs are

$$\hat{X}_{out} = (c + g_x) \hat{X}_m^{NLA} + x + \hat{X}_n \quad (5.17)$$

$$\hat{P}_{out} = (d + g_y) \hat{P}_m^{NLA} + y + \hat{P}_n \quad (5.18)$$

Under the unitary-gain condition, we get

$$g_x = \frac{\langle \hat{X}_{out} \rangle - x}{g_f \langle \hat{X}_m \rangle} - c \quad (5.19)$$

$$g_y = \frac{\langle \hat{P}_{out} \rangle - y}{g_f \langle \hat{P}_m \rangle} - d \quad (5.20)$$

$$V(\hat{X}_{out}) = (c + g_x)^2 g_f^2 * V(\hat{X}_m) + V(\hat{X}_n) \quad (5.21)$$

$$V(\hat{P}_{out}) = (d + g_y)^2 g_f^2 * V(\hat{P}_m) + V(\hat{P}_n) \quad (5.22)$$

Then the noise variances of output state can be expressed as

$$V(\hat{X}_{out}) = \frac{\left(\langle \hat{X}_{out} \rangle - x\right)^2}{g_f \langle \hat{X}_m \rangle^2} * V(\hat{X}_m) + V(\hat{X}_n) \quad (5.23)$$

$$V(\hat{P}_{out}) = \frac{\left(\langle \hat{P}_{out} \rangle - y\right)^2}{g_f \langle \hat{P}_m \rangle^2} * V(\hat{P}_m) + V(\hat{P}_n) \quad (5.24)$$

The formulas show that the effect of the NLA is equivalent to enhance the EPR entanglement, therefore our scheme in virtue of probability filter can realize high-fidelity quantum squeezing gate without limited entanglement. The fidelity limit is obtained in a heralded quantum squeezing gate with the NLA gain tended to infinity ( $g_f \rightarrow \infty$ ).

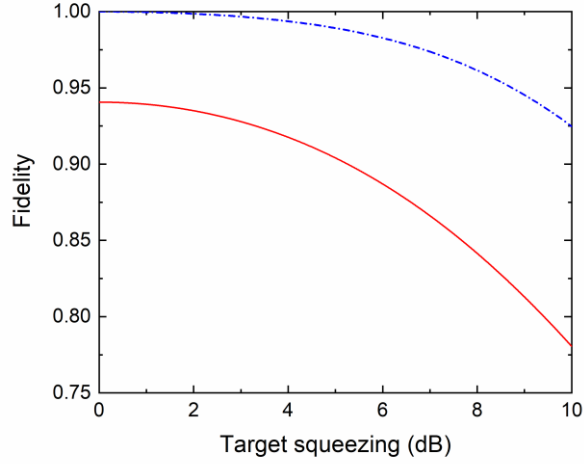

Fig. 5 Fidelity of a heralded and deterministic quantum squeezing gate. The blue dotted line is fidelity of a heralded quantum squeezing gate. The red line is fidelity of deterministic quantum squeezing gate.

Fidelities of a heralded and deterministic quantum squeezing gate are shown in Fig. 5, in which a pair of 12 dB-entangled EPR beams are taken into account. The blue dotted line is the fidelity limit of the heralded quantum squeezing gate with the NLA gain  $g_f \rightarrow \infty$ . The red line is fidelity of deterministic quantum squeezing gate in our scheme without NLA ( $g_f=1$ ). We find the unit fidelity can be realized beyond the auxiliary EPR entangled state limitation. Even when the target squeezing is set up to 10 dB, the calculated fidelity is still above 92%, much better than deterministic results. Thus, in virtue of the probability filter, our scheme expects to achieve higher fidelity with high success probability [9].

#### **B. Scheme of a heralded quantum squeezing gate based on ancillary squeezed state.**

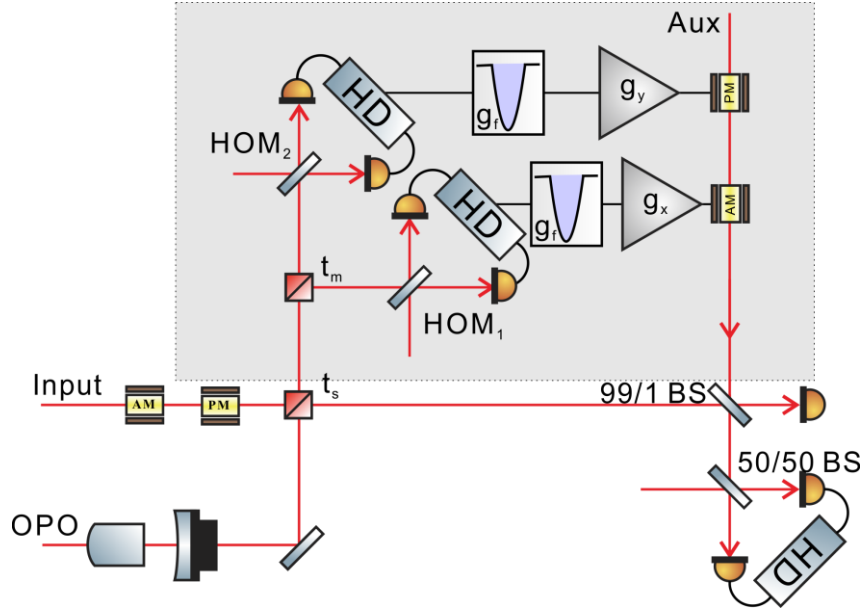

Fig. 6 Experimental scheme of the heralded squeezing gate with single beam of squeezed state.

Experimental scheme of the heralded squeezing gate with single beam of squeezed light is shown in Fig. 6. An input state is mixed with an ancillary squeezed state on a beam splitter with transmissivity  $t_s$ . The reflected mode and transmitted mode can be expressed to be:

$$\hat{a}_r = \sqrt{1-t_s} \hat{a}_{in} + \sqrt{t_s} \hat{a}_{sq} \quad (5.25)$$

$$\hat{a}_t = \sqrt{t_s} \hat{a}_{in} - \sqrt{1-t_s} \hat{a}_{sq} \quad (5.26)$$

Where  $\hat{a}_{in}$  and  $\hat{a}_{sq}$  are the input state and ancillary squeezed state, respectively.

The reflected mode is fed through an unbalanced homodyne detection (HOM) with a split of  $t_m$  that performs simultaneous measurements on the mode's amplitude and phase quadratures. The measurement outcomes can be expressed as:

$$\hat{X}_m = \sqrt{t_m} \hat{X}_v - \sqrt{1-t_m} \sqrt{1-t_s} \hat{X}_{in} - \sqrt{1-t_m} \sqrt{t_s} \hat{X}_{sq} \quad (5.27)$$

$$\hat{P}_m = \sqrt{1-t_m} \hat{P}_v + \sqrt{1-t_s} \sqrt{t_m} \hat{P}_{in} + \sqrt{t_s} \sqrt{t_m} \hat{P}_{sq} \quad (5.28)$$

Where  $\hat{X}$  and  $\hat{P}$  are amplitude and phase quadrature operators.  $\hat{X}_v$  and  $\hat{P}_v$  are the induced vacuum fluctuation caused by beam splitter.

Then we can express the transmitted mode as a function of the measured quadrature  $(\hat{X}_m, \hat{P}_m)$  via

$$\hat{X}_t = c\hat{X}_m + x + \hat{X}_n \quad (5.29)$$

$$\hat{P}_t = d\hat{P}_m + y + \hat{P}_n \quad (5.30)$$

Where

$$c = \frac{\sqrt{t_s(1-t_m)(1-t_s)}(e^{-2r_{ax}} - 1)}{t_m + (1-t_m)(1-t_s + t_s e^{-2r_{ax}})} \quad (5.31)$$

$$x = (\sqrt{t_s} + c\sqrt{(1-t_s)(1-t_m)})\langle \hat{X}_{in} \rangle \quad (5.32)$$

$$V(\hat{X}_n) = \frac{1 + (e^{2r_{ax}} - 1)t_s t_m}{t_s - t_s t_m + e^{2r_{ax}}(1 - t_s + t_s t_m)} \quad (5.33)$$

$$d = \frac{\sqrt{t_s t_m(1-t_s)}(1 - e^{2r_{ay}})}{(1-t_m) + t_m(1-t_s) + t_s t_m e^{2r_{ay}}} \quad (5.34)$$

$$y = (\sqrt{t_s} - d\sqrt{t_m(1-t_s)})\langle \hat{P}_{in} \rangle \quad (5.35)$$

$$V(\hat{P}_n) = \frac{t_s - t_s t_m + e^{2r_{ay}}(1 - t_s + t_s t_m)}{1 + (e^{2r_{ay}} - 1)t_s t_m} \quad (5.36)$$

After that, we implement the noiseless linear amplifier (NLA) operation on the measured outcomes of  $\hat{X}_m$  and  $\hat{P}_m$ . Then we transform  $\hat{X}_m$  into  $\hat{X}_m^{NLA}$  and  $\hat{P}_m$

$$\text{into } \hat{P}_m^{NLA} : \quad \langle \hat{X}_m^{NLA} \rangle = g_f * \langle \hat{X}_m \rangle, \quad \hat{X}_m^{NLA} = g_f * \hat{X}_m, \quad \langle \hat{P}_m^{NLA} \rangle = g_f * \langle \hat{P}_m \rangle,$$

$$\hat{P}_m^{NLA} = g_f * \hat{P}_m.$$

Finally, the rescaled signal is feedback into the amplitude modulator and phase modulator to displacement field, and the outputs are

$$\hat{X}_{out} = (c + g_x)\hat{X}_m^{NLA} + x + \hat{X}_n \quad (5.37)$$

$$\hat{P}_{out} = (d + g_y)\hat{P}_m^{NLA} + y + \hat{P}_n \quad (5.38)$$

a. Dual HOM ( $t_m=0.5$ )

In order to ensure that the squeezing operation is universal, the gate operates on the unity-gain condition; that is,  $\langle \hat{X}_{out} \rangle = e^{-r_i} \langle \hat{X}_{in} \rangle, \langle \hat{P}_{out} \rangle = e^{r_i} \langle \hat{P}_{in} \rangle$ . Under this condition,

we get

$$g_x = \frac{-e^{-2r_i} + \sqrt{t_s} + (1 - g_f)c\sqrt{(1-t_s)(1-t_m)}}{g_f\sqrt{(1-t_s)(1-t_m)}} \quad (5.39)$$

$$g_y = \frac{e^{2r_t} - \sqrt{t_s} + (1 - g_f)d\sqrt{t_m(1-t_s)}}{g_f\sqrt{t_m(1-t_s)}} \quad (5.40)$$

$$V(\hat{X}_{out}) = \left( \frac{e^{-r_t} - \sqrt{t_s} - c\langle\hat{X}_m\rangle}{\langle\hat{X}_m\rangle} \right) * \frac{V(\hat{X}_m)}{g_f} + V(\hat{X}_n) \quad (5.41)$$

$$V(\hat{P}_{out}) = \left( \frac{e^{r_t} - \sqrt{t_s} + d\langle\hat{P}_m\rangle}{\langle\hat{P}_m\rangle} \right)^2 * \frac{V(\hat{P}_m)}{g_f} + V(\hat{P}_n) \quad (5.42)$$

The formula show that fidelity can always be optimized by manipulating the values of  $t_s$  and  $t_m$ . In addition, the fidelity can be also improved by increasing the filter strength at the expense of a lower success probability for given target squeezing and squeezed ancilla.

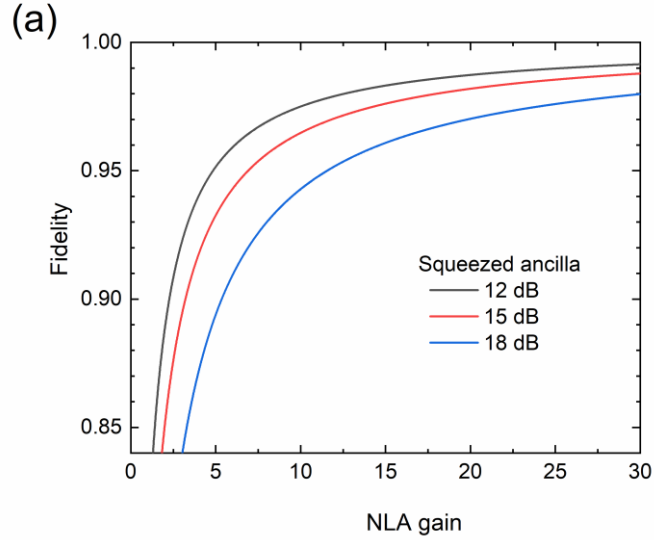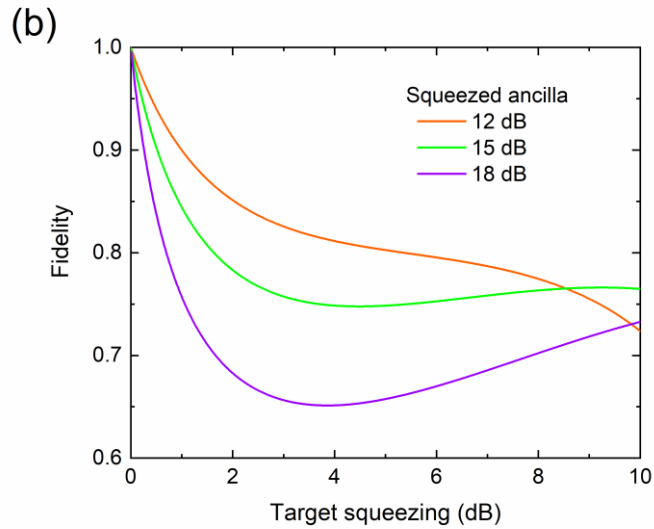

Fig. 7 Fidelities as a function of NLA gain (a) and target squeezing (b), respectively. (a) Dependence of fidelity on NLA gain for different the level of squeezed ancilla. At the target squeezing of -5 dB, curves black, red and blue show the numerical results with the auxiliary resource of -12 dB, -15 dB and -18 dB, respectively. (b) Fidelities as a function of the level of target squeezing at different squeezed ancilla when there is no noiseless linear amplifier (NLA) operation ( $g_f=1$ ).

Fidelities as a function of NLA gain at squeezed ancilla of -12 dB, -15 dB and -18 dB are shown in Fig. 7. The unit fidelity for any target squeezing is achievable with a sufficiently large filter strength at the expense of a lower success probability. However, when the probability of success is 1 (there is no NLA operation), the fidelity decreases with the improvement of squeezed ancilla. This is because the anti-squeezed variance increases with the improvement of squeezed degree.

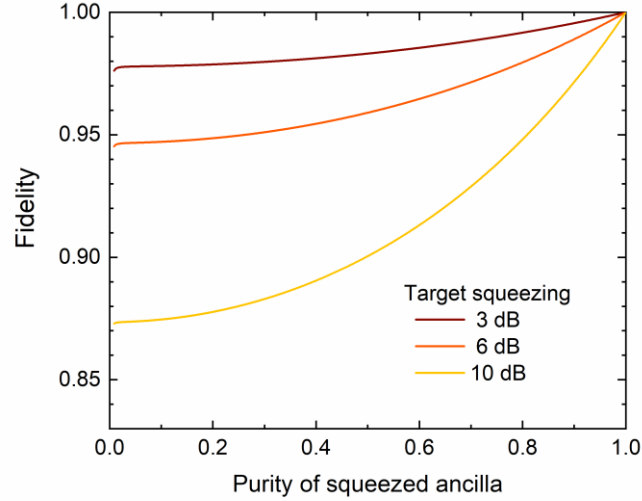

Fig. 8 Influence of the purity of the auxiliary squeezed state on the fidelity with a sufficiently large filter strength at squeezed ancilla of -12 dB.

When the purity of the auxiliary squeezed state is 1, the anti-squeezing variance is minimum at a specific squeezing factor. With the increase of the purity, the anti-squeezing variance increases. The influence of the purity of the auxiliary squeezed state on the fidelity is shown in Fig. 8. The fidelity of the squeezing gate decreases as the purity of the auxiliary squeezing state decreases, and the higher the target squeezing level is, the more obvious the influence on the purity is.

b. Single HOM ( $t_m=1$ )

$$g_y = \frac{\sqrt{1-t_s}(1+(e^{2r_{ay}}-1)g_ft_s)}{\sqrt{t_s}(g_f+(e^{2r_{ay}}-1)g_ft_s)} \quad (5.43)$$

$$V(\hat{X}_{out}) = t_s + (1-t_s)e^{-2r_{ax}} \quad (5.44)$$

$$V(\hat{P}_{out}) = \frac{1 + (e^{2r_{ay}} g_f - 1)t_s}{t_s g_f (1 + (e^{2r_{ay}} - 1)t_s)} \quad (5.45)$$

We can see that fidelity of the squeezing operation using squeezed state as an auxiliary resource is higher than that using EPR state. However, such a quantum squeezing gate containing single HOM cannot be used to implement complex operations.

In summary, the squeezing transformation that exploits an ancillary squeezed state as a resource cannot implement complex operations, including the squeezing operation and Fourier operation, at  $t_m=1$ . However, at  $t_m \neq 1$ , the high anti-squeezing variance of ancillary squeezed state restricts the improvement of the fidelity of squeezing gate based on the protocol of single auxiliary squeezed beam. The fidelity of the squeezing operation can be improved by using an NLA operation at the expense of a lower success probability.

#### Reference:

1. Z. Li, W. Ma, W. Yang, Y. Wang, and Y. Zheng, "Reduction of zero baseline drift of the Pound–Drever–Hall error signal with a wedged electro-optical crystal for squeezed state generation," *Opt. Lett.* **41**, 3331 (2016).
2. S. Shi, Y. Wang, W. Yang, Y. Zheng, and K. Peng, "Detection and perfect fitting of 13.2 dB squeezed vacuum states by considering green-light-induced infrared absorption," *Opt. Lett.* **43**, 5411-5414 (2018).
3. X. Sun, Y. Wang, L. Tian, Y. Zheng, and K. Peng, "Detection of 13.8 dB squeezed vacuum states by optimizing the interference efficiency and gain of balanced homodyne detection," *Chin. Opt. Lett.* **17**, 072701 (2019).
4. H. Zhou, W. Wang, C. Chen, and Y. Zheng, "A low-noise, large-dynamic-range-enhanced amplifier based on JFET buffering input and JFET bootstrap structure," *IEEE Sens. J.* **15**, 2101-2105 (2015).
5. H. Vahlbruch, M. Mehmet, S. Chelkowski, B. Hage, A. Franzen, N. Lastzka, and R. Schnabel, "Observation of squeezed light with 10-dB quantum-noise reduction," *Phys. Rev. Lett.* **100**, 033602 (2008).
6. M. Mehmet, S. Ast, T. Eberle, S. Steinlechner, H. Vahlbruch, and R. Schnabel, "Squeezed light at 1550 nm with a quantum noise reduction of 12.3 dB," *Opt. Express* **19**, 25763-25772 (2011).
7. R. Ukai, N. Iwata, Y. Shimokawa, S. C. Armstrong, A. Politi, J. I. Yoshikawa, P. van Loock, and A. Furusawa, "Demonstration of unconditional one-way quantum computations for continuous variables," *Phys. Rev. Lett.* **106**, 240504 (2011).
8. S. Hao, X. Deng, X. Su, X. Jia, C. Xie, and K. Peng, "Gates for one-way quantum computation based on Einstein-Podolsky-Rosen entanglement," *Phys. Rev. A* **89**, 032311 (2014).
9. J. Zhao, K. Liu, H. Jeng, M. Gu, J. Thompson, P. K. Lam, and S. M. Assad, "A high-fidelity heralded quantum squeezing gate," *Nat. Photonics* **14**, 306-309 (2020).
